# Supplementary material for: Curated Collaborative AI Edge with Network Data Analytics for B5G/6G Radio Access Networks
Source: arXiv:2507.01994 source file (2026-11-25)
Supplement: Supplementary file 1 [file supplementary.tex]

\documentclass[12pt, draftclsnofoot, onecolumn]{IEEEtran}
\usepackage{setspace}
\usepackage[margin=1in]{geometry} % Adjusts to IEEE’s required 6.5in text width
\doublespacing
  % Sets 6.5-inch text width on standard 8.5in x 11in paper 

% \doublespacing  % Applies double-spacing to the document

\geometry{textwidth=6.5in}  % Set line length to 6.5 inches
\doublespacing  % Enable double-spacing \documentclass[lettersize,journal]{IEEEtran}
% \documentclass[lettersize,journal]{IEEEtran}
% \usepackage{amsmath,amsfonts}
% \usepackage{algorithmic}
% \usepackage{algorithm}
% \usepackage{array}

% \documentclass[lettersize,journal]{IEEEtran}

% ====== Core Packages ======
\usepackage{amsmath,amssymb,amsfonts}
\usepackage{graphicx}
\usepackage{xcolor}
\usepackage{cite}
\usepackage{url}
\usepackage{verbatim}
\usepackage{tikz}
\usepackage{stfloats}
\usepackage{multirow}
\usepackage{makecell}
\usepackage{soul}
\usepackage{orcidlink}

% ====== Algorithm Setup ======
\usepackage[ruled,vlined,linesnumbered,longend,resetcount]{algorithm2e}

% ====== Figure/Caption Setup ======
\usepackage[labelsep=period]{caption}
\usepackage{subcaption} % Modern subfigures (remove if using subfig)

% ====== Custom Commands ======

% ====== Document Settings ======
\UseRawInputEncoding

\begin{document}

% Main title
\title{Curated Collaborative AI Edge with Network Data Analytics for B5G/6G RAN}
\maketitle  % Print the title

% Supplementary Material Title
\begin{center}
    \textbf{Supplementary materials}
\end{center}
\vspace{1em}  % Adds some space before starting the next section

% \begin

\section{Logical clustering within each Edge Cloud}

The proposed Curated Collaborative Learning (CCL) framework strategically selects collaborating partners, a process that is not feasible at the Edge Cloud (EC) level for traffic prediction due to the similarity in average traffic patterns among ECs. To fully leverage its potential, CCL is applied at the logical cluster level, where each EC is divided into $m$ logical clusters, as detailed in the main manuscript. The selection process follows the Algorithm \ref{algS1} provided below and uses the following Eq. \ref{eq1} for calculating the Pearson Correlation Coefficient (PCC).

\begin{equation}
p_{x,y} = \frac{{}\sum_{i=1}^{h} (x_i - \overline{x})(y_i - \overline{y})}
{\sqrt{\sum_{i=1}^{h} (x_i - \overline{x})^2  \sum_{i=1}^{h}(y_i - \overline{y})^2}}
\label{eq1}
\end{equation}

Here, $\overline{x}$ and $\overline{y}$ are the arithmetic mean of hourly traffic of $P_{i}$ and $P{j}$ over $h$ hours, respectively.

\begin{algorithm}[t]
{
\caption{Urbanflow Peak-time Clustering (UPC) for logical clustering}
\label{algS1}
\small
    \LinesNumbered
    \SetKwInOut{Input}{Input} 
    \SetKwInOut{Output}{Output}
    \label{algo1}
    \Input{Set of base stations $B$ in an edge; hours $H = \{0, \raisebox{0.5ex}{\dots}, 23\}$.}
    \Output{$m$ logical clusters of an edge.}    
    \BlankLine
        
    \tcp{Step 1: Grouping BSs based on peak traffic hours}
    \BlankLine
    \For {each base station $b \in B$}{            
        $i = \arg\max_{h \in H} \{b.\text{traffic}(h)\}$ \\
        $P_i \leftarrow P_i \cup \{b\}$\\
    }
  
    \For {$i \gets 0$ to $|H|-1$}{
        \If{$P_i \neq \emptyset$}{
            \For {$h \gets 0$ to $|H|-1$}{
                $P_i.\text{traffic}(h) \gets \frac{\sum_{\forall b \in P_i}{b.\text{traffic}(h)}}{|P_i|}$ \\
            }
        }
    }
    \BlankLine
    \tcp{Step 2: Calculate pairwise PCC among all $P_i$}
    \BlankLine
    \For {$i \gets 0$ to $|H|-1$}{
        \For {$j \gets 0$ to $|H|-1$}{
            \If{$P_i \neq \emptyset$ and $P_j \neq \emptyset $}{
                $p_{i,j} \gets$ PCC between $P_i$ and $P_j$ using Eq. (\ref{eq1}) \\
            }\Else{
                $p_{i,j} \gets 0$ \\
            }
        }
    }

    $\mathcal{L} \gets \mathrm{Consolidating}(P_{i (\forall i \in H)}, m)$ \tcp{Consolidating into $m$ logical clusters that maximize the average PCC among the clusters.}
    
    \Return $\mathcal{L}$ \tcp{Return the final set of $m$ logical clusters.}
}
\end{algorithm}

\newpage

\section{Dataset and experimental setup}

The available cellular dataset does not employ any EC architecture. Therefore, k-means clustering is applied to do so via the Elbow method. This method relies on the calculation of the Sum of Squared Errors (SSE) between each point and the centroid at each EC for various values of $k$. As $k$ increases, the SSE tends to decrease, reflecting the improvement in clustering. However, there comes a point where the reduction in error diminishes significantly with further increases in $k$. This pivotal juncture forms what is known as the elbow, indicating the optimal value of $k$ for the ECs. The SSE is calculated as:

\begin{equation}
\text{SSE} = \sum_{i=1}^{k} \sum_{x \in C_i} \| x - \mu_i \|^2
\end{equation}

where \( k \) is the number of ECs, \( C_i \) is the set of points in the \( i \)-th EC, \( \mu_i \) is the centroid of the \( i \)-th EC, \( x \) represents each BS location in the \( i \)-th EC, and \( \| x - \mu_i \|^2 \) is the squared Euclidean distance between a data point i.e., BS location \( x \) and the centroid \( \mu_i \). As depicted in Fig. S1, the elbow curve illustrates that the optimal value of $k$ is 11. This conclusion is drawn from observing a significant reduction in the SSE as $k$ increases from 1 to 11, beyond which the decrease in error becomes marginal. Therefore, it can be inferred that 1072 BSs can be effectively assigned to 11 ECs. Fig. 4 in the original manuscript provides a visual representation of the physical clustering outcome on the OpenStreetMap of the actual city. 

\begin{figure}[t]
\centering
\includegraphics[width=3.0in]{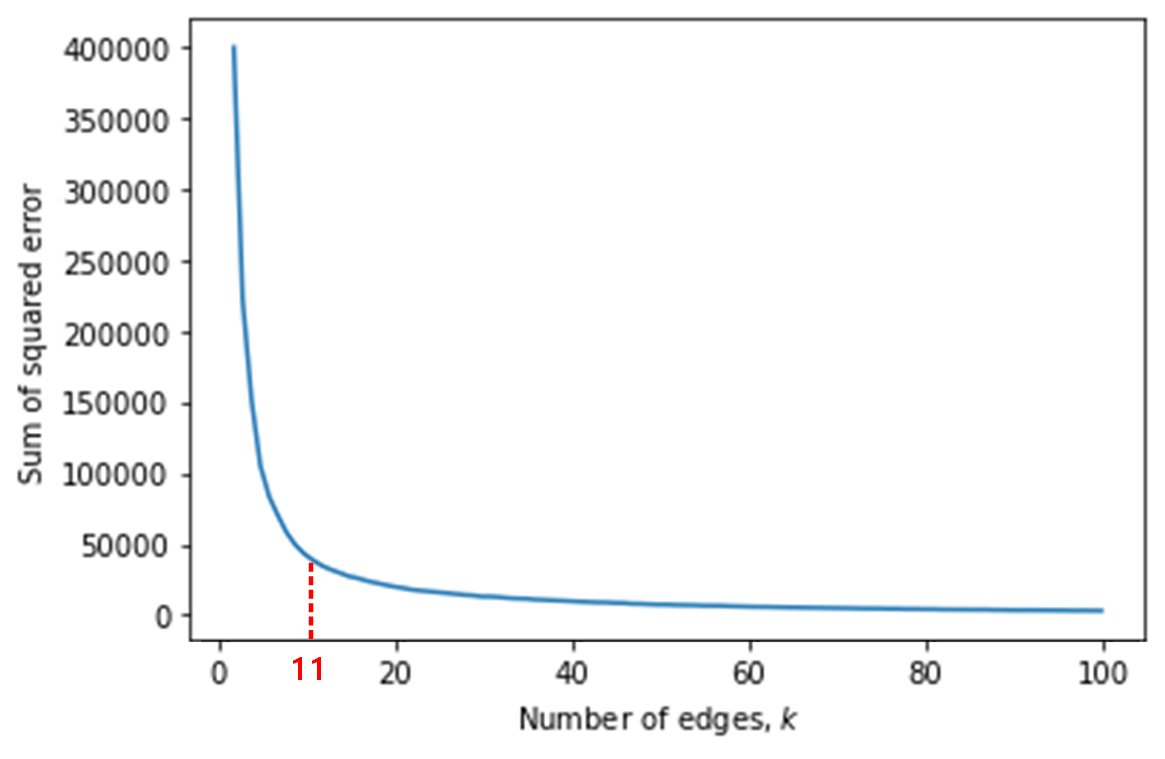}
\caption{Determining the optimal number of edge clouds via the Elbow method.}
\label{fig_4}
\end{figure}

\newpage

\section{Hyperparameters for MSTNet training}

\renewcommand{\thetable}{S\arabic{table}} % Change table numbering to S1, S2, ...

\begin{table}[h]
\caption{Hyperparameter values for MSTNet training.}
\centering
\renewcommand{\arraystretch}{1.2} % Adjust row spacing for better readability
\begin{tabular}{l p{10cm} c }
\hline
\textbf{Parameter} & \textbf{Description} & \textbf{Value} \\
\hline
Epoch & The number of complete passes through the training dataset. & 1000 \\
\hline
Batch size & the number of training examples utilized in one iteration. & 32 \\
\hline
Learning rate & the step size at each iteration while moving toward a minimum of the loss function. & 0.001 \\
\hline
Dropout & The fraction of input units dropped to prevent overfitting. & 0.2 \\
\hline
Time interval (min) & The time duration (in minutes) between successive data points. & 10 \\
\hline
Dilated factor & A factor for expanding the model's receptive field, expressed as \(2^i\). & \(2^i\) \\
\hline
\end{tabular}
\label{tab:S1}
\end{table}

% Start of supplementary content
\section{Ablation Studies}

\subsection{Ablation studies for collaboration strategy}
A set of experiments is conducted to identify the most effective collaboration strategy among logical clusters for $\hat{\tau}$ and $\hat{u}$ predictions. As mentioned earlier, this strategy involves identifying i) whom to collaborate with, ii) determining when to collaborate, and iii) what parameters to collaborate with. The following paragraphs present ablation studies for each of the three aspects, varying one aspect at a time while keeping the other two constant, and \(q=3 \) is utilized throughout.

A variety of collaborative partnerships can be formed among the logical clusters. Scenarios include IdEL (no collaboration), collaboration among all clusters regardless of their traffic patterns, collaboration among clusters with contrasting patterns or negative correlation, and collaboration only among those exhibiting highly positive correlation surpassing a predefined threshold. Table \ref{tab_3} displays the average MAE across all logical clusters in these four scenarios. Results show that IdEL (no collaboration) yields satisfactory outcomes but struggles with out-of-distribution data. Collaboration with all clusters or negatively correlated clusters degrades performance due to mixed and contradictory patterns. Optimal results are achieved by collaborating with highly correlated clusters.

\begin{table*}[t]
\caption{MAE comparison for various collaboration partners. Here, the collaboration frequency threshold is 30\%, and the collaborating parameters are from TCN-LSTM.}
\centering
\begin{tabular}{lcc}
\hline
\rule{0pt}{10pt} \multirow{2}{*}{\textbf{Collaborating partnerships}} & \multicolumn{1}{c}{\textbf{MAE in}} & \multicolumn{1}{c}{\textbf{MAE in}} \\
  & \multicolumn{1}{c}{\textbf{user count}} & \multicolumn{1}{c}{\textbf{traffic (GBs)}} \\
\hline
\rule{0pt}{10pt} No collaboration & 20 & 2.96 \\
\hline
\rule{0pt}{10pt} All collaborate & 29 & 3.3 \\
\hline
\rule{0pt}{10pt} Cross-correlated & 35 & 3.6 \\
\hline
\rule{0pt}{10pt} Proposed (correlation $>$ 95\%) & \textbf{14} & \textbf{2.19} \\
\hline
\end{tabular}
\label{tab_3}
\end{table*}

\begin{figure}[!t]
\centering
\begin{minipage}{0.37\textwidth}
   \includegraphics[width=\textwidth]{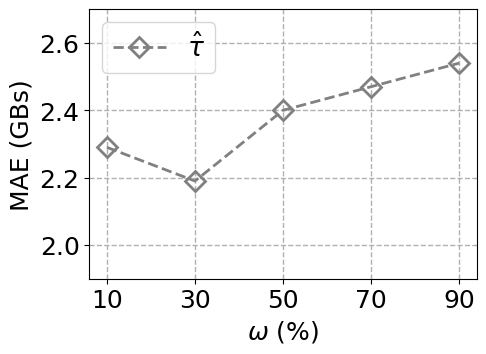}
   \caption*{{(a) BS traffic prediction $\hat{\tau}$}}
   \label{fig3a} 
\end{minipage} 
\hfill
\begin{minipage}{0.37\textwidth}
   \includegraphics[width=\textwidth]{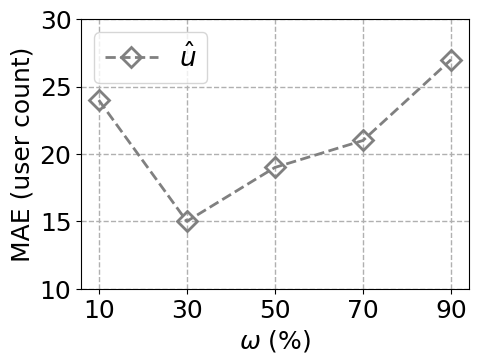}
   \caption*{{(b) BS user count $\hat{u}$}}
   \label{fig3b}
\end{minipage}
\hfill
   \caption{MAE for prediction tasks over varying collaboration frequency threshold $\omega$.}
    \label{fig_9}
% \vspace{-0.18cm}

\end{figure}

The optimal collaboration frequency is determined through extensive experiments by varying the threshold for validation loss changes and evaluating the corresponding model performance in terms of MAE. As shown in Fig. \ref{fig_9}, the CCL performance depends on the chosen collaboration frequency threshold. For instance, when the change in validation loss is set to less than 10\% of its previous value, the model achieves a specific MAE. Similarly, thresholds of 20\% and 30\% are tested, with corresponding MAEs measured to identify the best configuration. Frequent collaborations (e.g., with a low threshold) slow down convergence and lead to premature parameter sharing, while a threshold of 30\% provides the optimal balance between accuracy and overhead. This indicates that the model has already learned meaningful insights and is ready to share. In some scenarios, minimizing overhead outweighs maximizing accuracy, favoring lower collaboration frequency for reduced computation with acceptable performance.

\begin{table}[t]
\caption{MAE comparison for various collaborating parameters. Here, the collaboration frequency threshold is 30\%, and collaborating with highly correlated ($>$ 95\%) logical clusters.}
\centering
\begin{tabular}{lcc}
\hline
\rule{0pt}{12pt}\multirow{2}{*}{\textbf{Collaborating parameters}} & \textbf{MAE in} & \textbf{MAE in} \\
\rule{0pt}{12pt} & \textbf{user count} & \textbf{traffic (GBs)} \\
\hline
\rule{0pt}{12pt} All & 34 & 3 \\
\hline
\rule{0pt}{12pt} MSP & 41 & 3.9 \\
\hline
\rule{0pt}{12pt} TCN-LSTM & \textbf{14} & \textbf{2.19} \\
\hline
\end{tabular}
\label{tab_4}
\end{table}

Demonstrating the impact of selecting parameters from collaborating models, experiments have been conducted with various combinations of shared parameters to assess performance in predicting future traffic and user counts. To recall, the model consists of three main components, including i) the TCN-LSTM block, ii) the RC, and iii) MSP branches for traffic and user count prediction. Table \ref{tab_4} presents a comparison of different parameter-sharing setups. In the first case, all parameters are shared; in the second, only branch weights are shared among collaborating clusters; and in the third, only the TCN-LSTM block parameters are shared. Results demonstrate that the model performs best when only the TCN-LSTM parameters are shared, as these parameters are minimally affected by backpropagation. This selective collaboration approach enhances generalization in one portion of the model, while branches keep biases, tailored to their respective logical clusters.

\subsection{Computational comparison of CCL with other learning}

The computational cost of different learning schemes was evaluated in terms of training time and convergence of validation loss on an RTX 4090 GPU. For training efficiency as shown in Fig. S3, CCL is 87.3\% faster than GL, completing training in 2,273 seconds compared to 17,865 seconds. FL further reduces training time by 10.8\% compared to CCL, while IdEL is the fastest, being 17.7\% faster than FL and 17.9\% faster than CCL due to its purely local training approach.

\begin{figure}[t]
\centering
\includegraphics[width=5.0in]{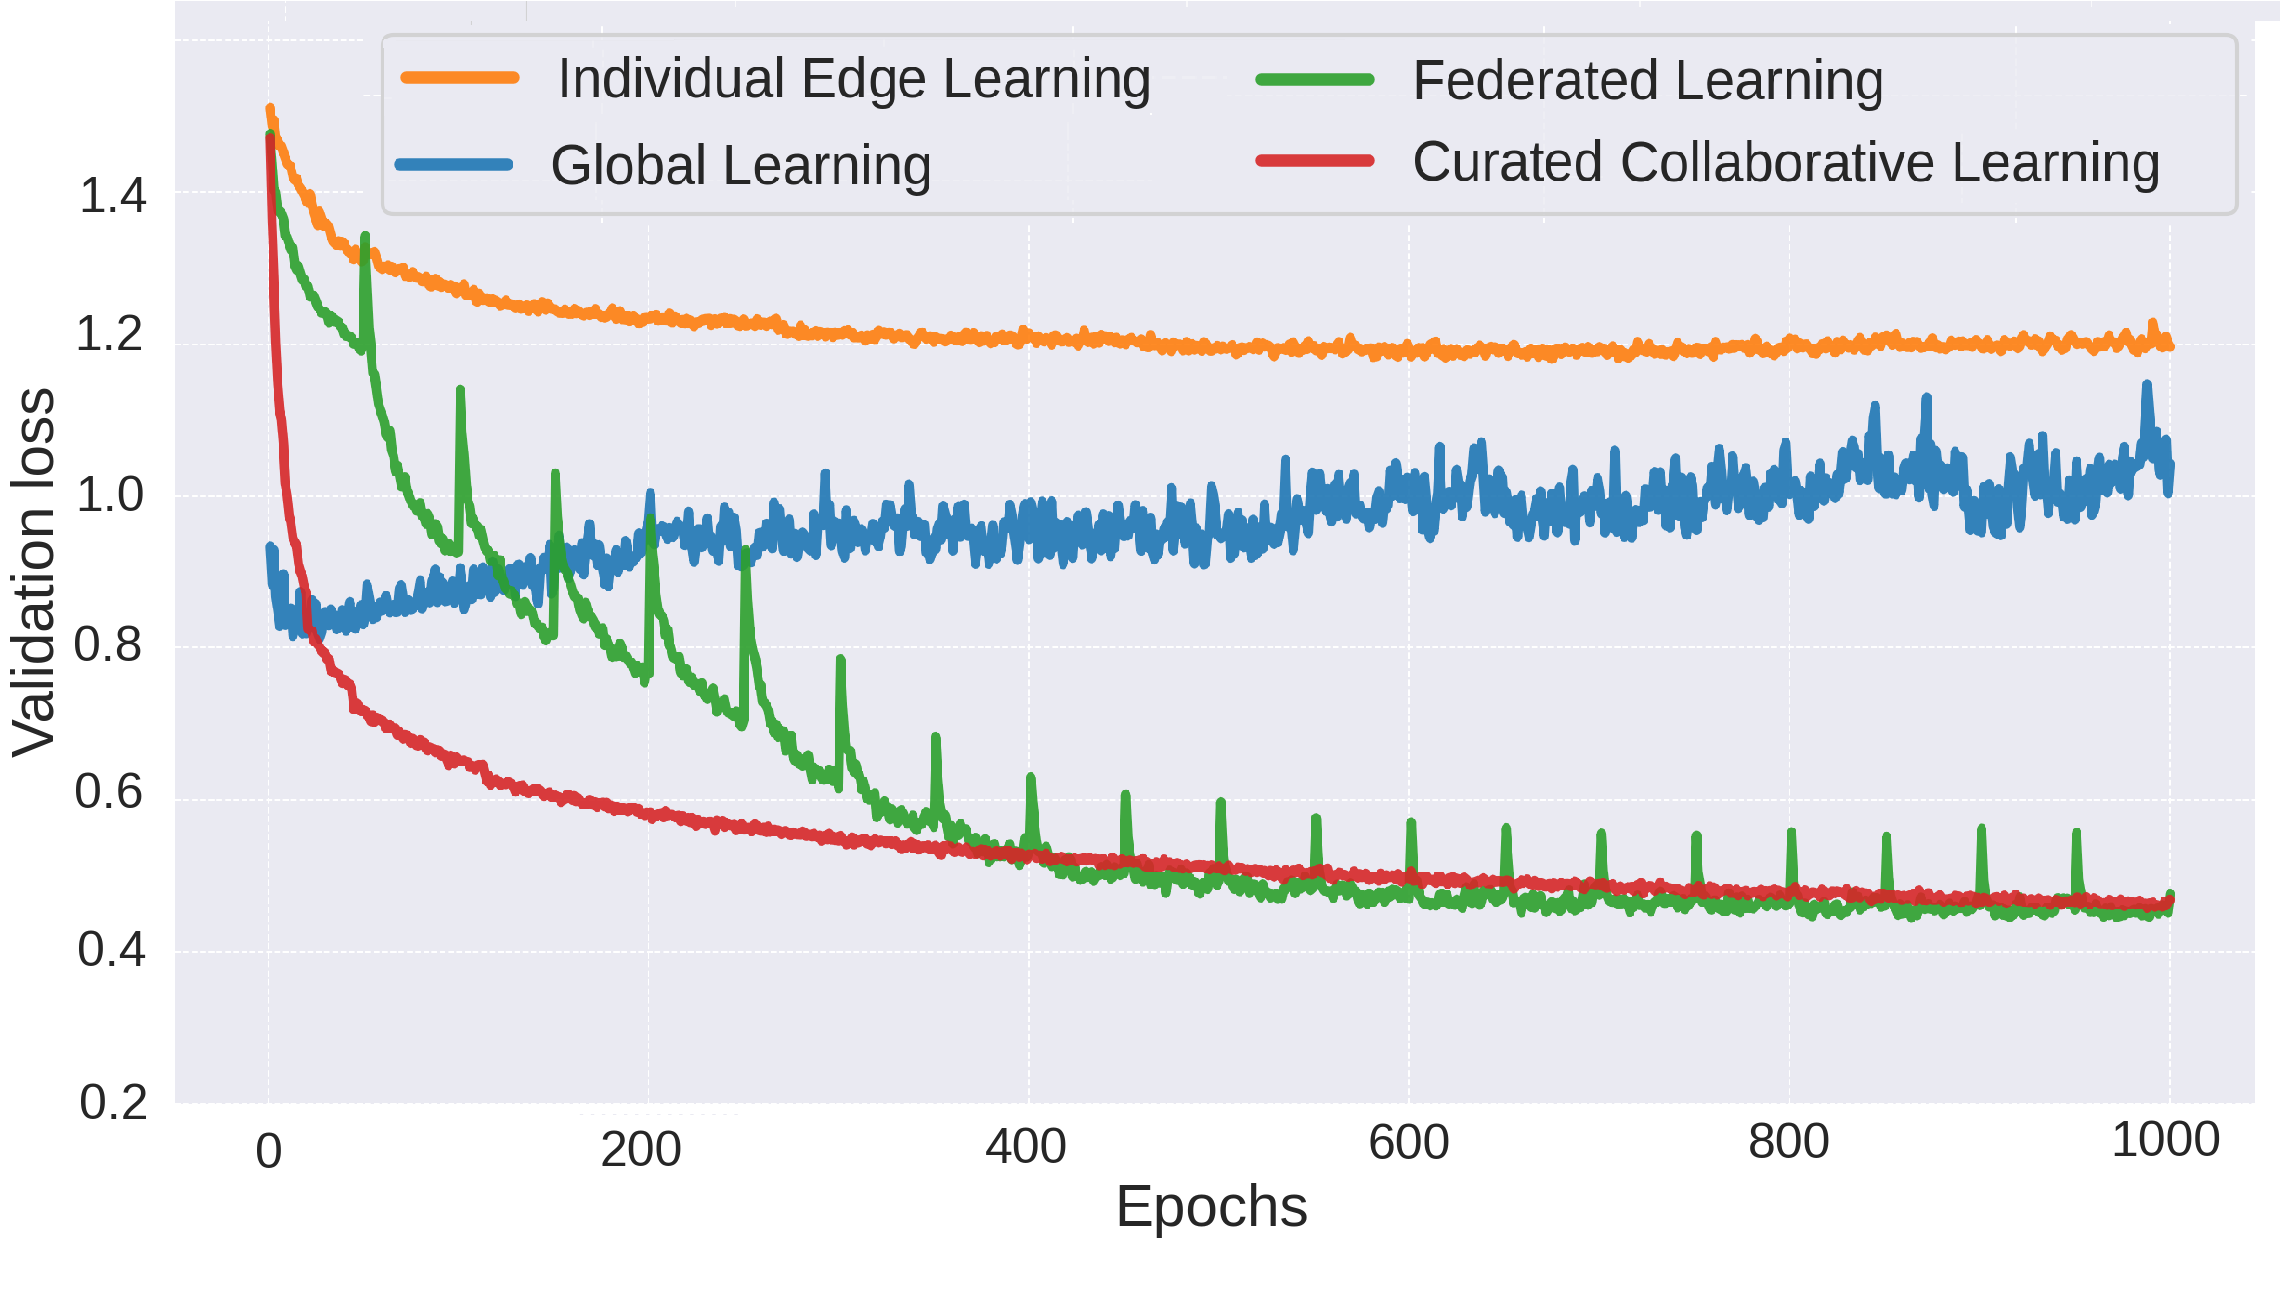}
\caption{Validation loss comparison of Global, Individual Edge, Federated, and Curated Collaborating learning.}
\label{fig_4}
\end{figure}
The validation loss trends across different learning paradigms highlight distinct convergence behaviors and generalization capabilities. CCL exhibits the fastest convergence, reaching 80\% of its final validation loss by epoch 200. In contrast, FL requires approximately 300 epochs to reach a similar level, making it 50\% slower than CCL. GL converges significantly later, around 500 epochs, making it 150\% slower than CCL, while IdEL fails to fully converge within the given training period.

Despite FL achieving a slightly lower final validation loss (≈0.42), its periodic spikes indicate instability, likely due to aggregation inconsistencies in federated averaging. CCL follows closely with a final validation loss of ≈0.45, but its smooth learning curve and stable convergence result in better generalization, as evidenced by a 40\% lower MAE on the test dataset compared to FL. GL (≈0.80) and IdEL (≈1.20) show significantly higher losses, demonstrating weak generalization and poor convergence. Thus, CCL emerges as the most effective approach, balancing fast convergence, stability, and superior test performance.

\subsection{Ablation studies for DUPS}

Fig. 10 in the main manuscript presents three edge clouds, $EC_{10}$, $EC_{3}$, and $EC_{11}$, representing high, moderate, and low traffic edges, respectively, to illustrate the effectiveness of the proposed DUPS under varying conditions. Several experiments have been conducted to determine the optimal configuration parameters for all three DRL environments, aimed at reducing the number of DU servers while maintaining fronthaul latency requirements. These parameters include $\alpha$, $\beta$ used in the reward function, and DU server capacity $d$.

\begin{figure}[!t]
\centering
\begin{minipage}{0.32\textwidth}
   \includegraphics[width=\textwidth]{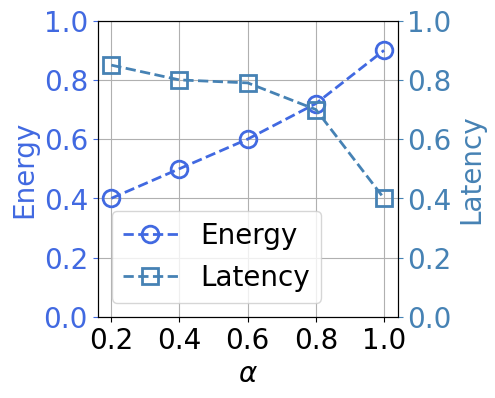}
   \caption*{(a) High traffic ($EC_{10}$)}
   \label{fig3a} 
\end{minipage} 
\hfill
\begin{minipage}{0.32\textwidth}
   \includegraphics[width=\textwidth]{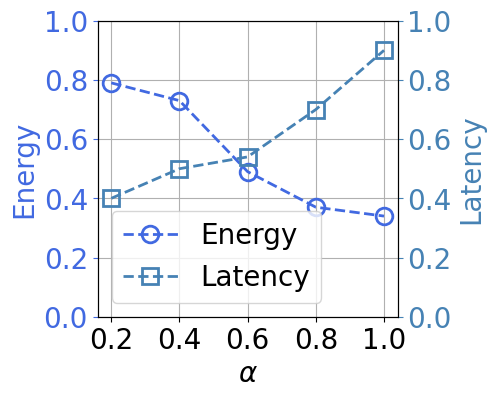}
   \caption*{{(b) Moderate traffic ($EC_3$)}}
   \label{fig3b}
\end{minipage}
\hfill
\begin{minipage}{0.32\textwidth}
   \includegraphics[width=\textwidth]{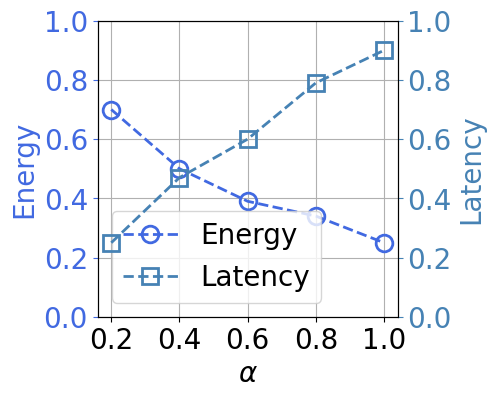}
   \caption*{(c) Low traffic ($EC_{11}$)}
   \label{fig3b}
\end{minipage}
    \caption{Energy-latency trade-off over varying the coefficient parameter $\alpha$ for contrast traffic intensive  edges.}
    %These three ECs are from our dataset, which includes a total of 11 ECs.
    \label{fig_10}
% \vspace{-0.18cm}

\end{figure}

Selecting an optimal value of \( \alpha \) is crucial for balancing energy and latency in the reward function, with fixed parameters \( \beta = 0.5 \) and $d$ = 192 GBs. Energy and latency are normalized between 0 and 1. For energy, 0 represents a DU server being off, while 1 represents 100\% CPU utilization, calculated using the energy model from \cite{r45}. For latency, 0 indicates the DU server is positioned very close to the RU of the BS, and 1 represents the maximum allowable FH latency of \( 50 \, \mu \text{sec} \). Fig. \ref{fig_10} compares these parameters across different \( \alpha \) values. For high-traffic edges, a higher \( \alpha \) prioritizes energy savings, allowing the system to tolerate greater latency. This encourages agents to turn off more servers, even at the cost of redirecting traffic and increasing latency. In contrast, in low-traffic regions with sparsely distributed BSs, a lower \( \alpha \) emphasizes latency, discouraging agents from redirecting traffic to distant DU servers, thereby ensuring better performance for the limited traffic.

\begin{figure}[!t]
\centering
\begin{minipage}{0.3\textwidth}
   \includegraphics[width=\textwidth]{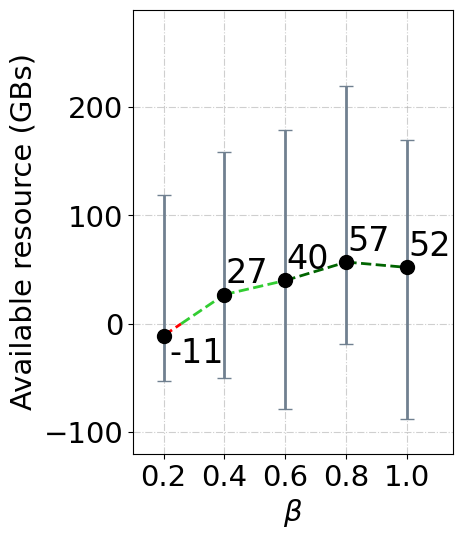}
   \caption*{(a) High traffic ($EC_{10}$)}
   \label{fig3a} 
\end{minipage} 
\hfill
\begin{minipage}{0.3\textwidth}
   \includegraphics[width=\textwidth]{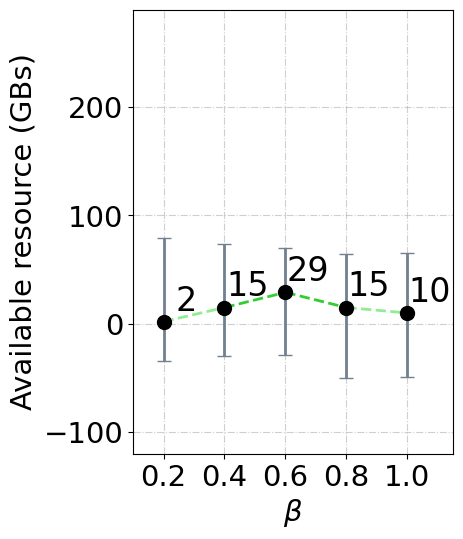}
   \caption*{(b) Moderate traffic ($EC_{3}$)}
   \label{fig3b}
\end{minipage}
\hfill
\begin{minipage}{0.3\textwidth}
   \includegraphics[width=\textwidth]{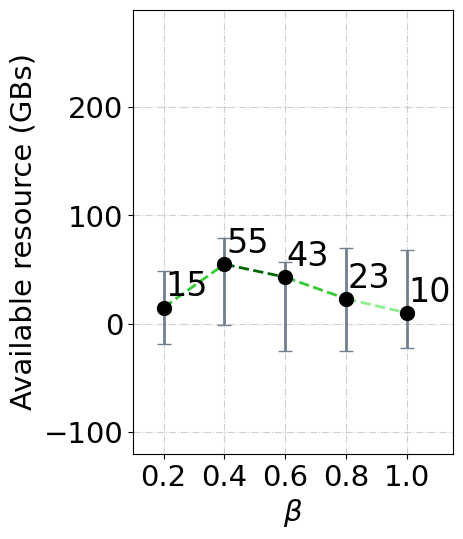}
   \caption*{(c) Low traffic ($EC_{11}$)}
   \label{fig3b}
\end{minipage}
    \caption{Average available (surplus+/shortage-) memory resource (GBs) over varying penalizing parameter $\beta$ for contrastive traffic edges. }%Bold center values represent the average surplus (green) or rejected (red) traffic during experiments with respective $\alpha$ from the previous figure.}
    \label{fig_11}
% \vspace{-0.18cm}

\end{figure}

The next parameter is $\beta$, which controls the penalty given to agents if they violate either the FH latency bound or redirect traffic to an already overloaded DU server, causing traffic to be rejected. Fig. \ref{fig_11} illustrates the effect of varying $\beta$ on the total capacity of DU servers offered by the DRL. For instance, if the DRL offers 15 DU servers, each with a capacity of 192 GBs, the total capacity would be $15 \times 192$ = 2.8 TBs. If the actual traffic for edge $EC_i$ is about 2.9 TBs, resulting in traffic rejection of 0.1 TBs. On the other hand, if the actual traffic is 2.2 TBs, there would be a surplus of 0.6 TBs offered by the DRL. This analysis is conducted with a fixed $\alpha$ of 0.8, 0.6, and 0.4 for the three edges $EC_{10}$, $EC_{3}$, and $EC_{11}$, respectively, while keeping  $d$ = 192 GBs. For a high-traffic edge $EC_{10}$, a higher $\beta$ is crucial because high-traffic edges are more likely to violate FH latency bounds or overload nearby servers when a DU server is turned off. Assigning a higher penalty discourages the DRL from actions that lead to traffic rejection, ensuring balanced server usage and better performance under heavy traffic loads. Conversely, in low-traffic edges, the risk of exceeding FH latency bounds or overloading servers is minimal due to the lighter load. Therefore, a lower $\beta$ allows the DRL to prioritize energy savings and reduce unnecessary penalties, enabling efficient use of resources without compromising service quality.

\begin{figure}[t]
\centering
\begin{minipage}{0.79\textwidth}
   \includegraphics[width=\textwidth]{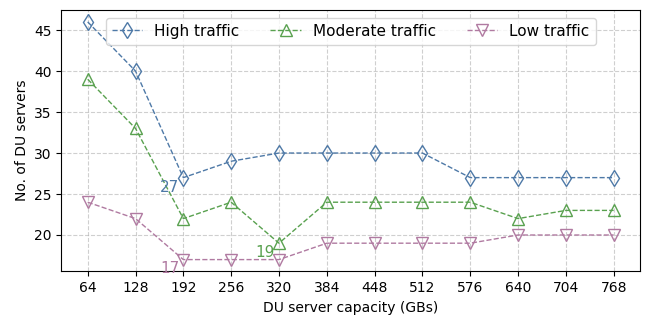}
   \caption*{{(a) Average number of DU servers.}}
   \label{fig3a} 
\end{minipage} 
\hfill
\begin{minipage}{0.79\textwidth}
   \includegraphics[width=\textwidth]{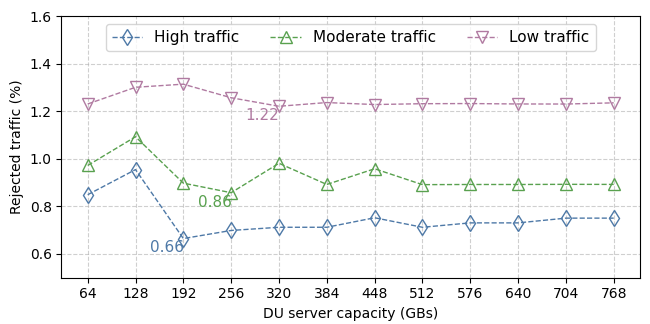}
   \caption*{{(b)  Rejected traffic (\%) of actual traffic.}}
   \label{fig3b}
\end{minipage}
    \caption{Effects on system availability with varying DU server capacity.}
   \label{fig_12} 
% \vspace{-0.18cm}

\end{figure}

Once the appropriate values of \( \alpha \) and \( \beta \) are determined, these parameters are used to identify optimal DU server capacities for each edge. Fig. \ref{fig_12} shows the performance of each edge in terms of the average number of DU servers and the percentage of rejected traffic across varying capacities. The high-traffic edge $EC_{10}$ achieves minimal DU servers and rejected traffic at  $d$ = 192 GBs, while the optimal capacities for $EC_{3}$ and $EC_{11}$ are $d$ = 256 GBs and 320 GBs, respectively. The primary objective is to minimize rejected traffic, as it directly impacts customer satisfaction and the credibility of the operators. Additionally, high-traffic edges benefit from smaller DU capacities to reduce overhead, whereas moderate and low-traffic edges require higher capacities to handle traffic fluctuations effectively.

    \bibliographystyle{IEEEtran}
    \bibliography{reference}

% \section{Pending tasks}
% \\
% \begin{itemize}
%     \item Model Fig. 3 enhancement. Submitted the initial draft to Dr. Raza for final touch ups. \\
%     \item Section 3D: DRL for DU Pooling: Writeup, and algorithm 4.  Submitted the initial draft to Dr. Josh for final touch ups. \\
%     \item Notation will be revised based on the changes in task 2.\\
% \end{itemize}

    % \newpage

\end{document}
